# Supplementary material for: Photoemission-based microelectronic devices
Source: arXiv:1512.02197 source file (2016-04-19)
Supplement: Supplementary file 1 [file SI.pdf]

# Supporting Information: Photoemission-based Microelectronic Devices

Figure S.1 shows the proposed electro-optical photoemission inspired by SERS in which the incoming laser intensity is enhanced by the designed cavities on the surface. Figure S.2 shows a proposed photoemission-based device, i.e. a photon-gate transistor. Figure S.3 shows our studied two-port device in more details. Two airbrdiges on the device's sides feed the suspending port with proper static polarities.

Figure S.4 depicts the measurement setup. The fabricated devices were packaged (using standard dual in-line packages) and wire-bonded (using a ball bonder) as shown in Fig. S.5. Coaxial cables and connectors were used to feed the device inside the vacuum chamber. Use of coaxial cables prevented any plasma formation around the cables, even with applied high voltages. The packages in Fig. S.5 are ordered from Spectrum Semiconductor Materials Inc. (Part. no. CCF00604).

To confirm the significant effect of the resonant surface, some non-resonant structures (simple flat structures) were fabricated on quartz as shown in Fig. S.6. The measured currents for all of these structures were less than 100 nA even with applied voltages above 100 V on either ports and with large laser illuminations greater than $1\,\mathrm{W/mm^2}$. Figure S.7 shows a sample of current measurements using theses devices. Quartz was chosen as the substrate for these flat structures to remove any possible substrate contributions in current measurements. We also tried to fabricate our resonant devices on quartz, but their fabrication was quite challenging since the pattern was too dense and the charge buildup on the isolator substrate distorted the Ebeam lithography repeatedly. Using conductive polymers as the charge dissipator layer did not solve the problem either. Figure S. 8 shows I-V curves of the flat port with different suspended port excitations and without the laser illumination. The conductivity change of the dark device is much smaller than the activated device.

---

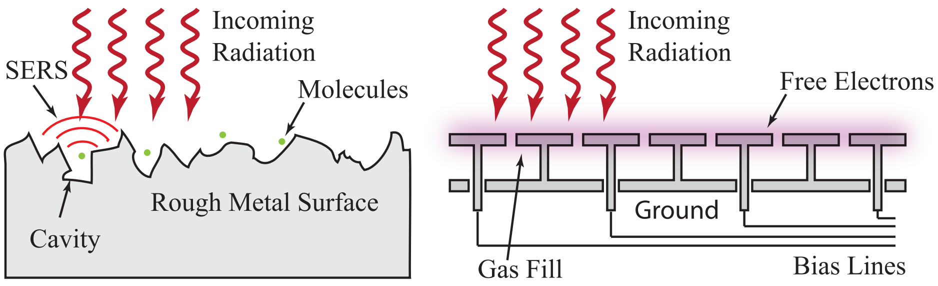


Figure S.1. The proposed electro-optical excitation concept. Inspired by SERS (left), the suggested concept is to activate the photoemission-based device using optical power pumping a designed resonant surface (right). The bias lines further reduce optical power requirements and provide photonic/electronic controllability.

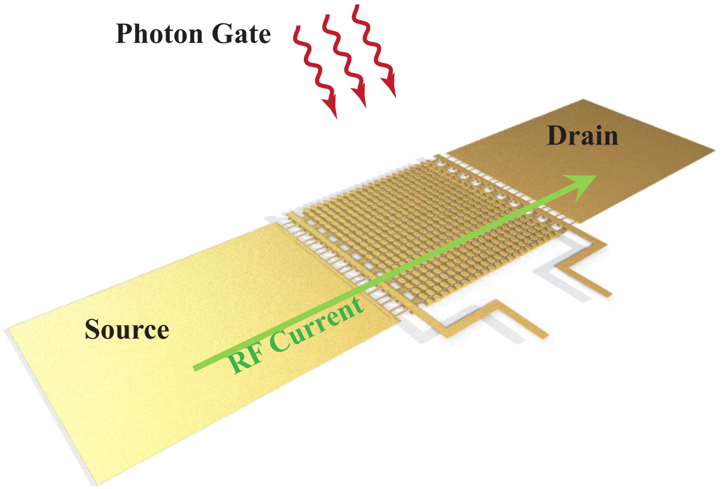


Figure S.2. Photoemission-based transistor. Biased resonant inclusions under illumination by a wavelength-tuned CW laser emit electrons. The free electrons can be manipulated electrically by proper applied voltages. The bias signal along with the incoming laser beam control the conductivity between source and drain.

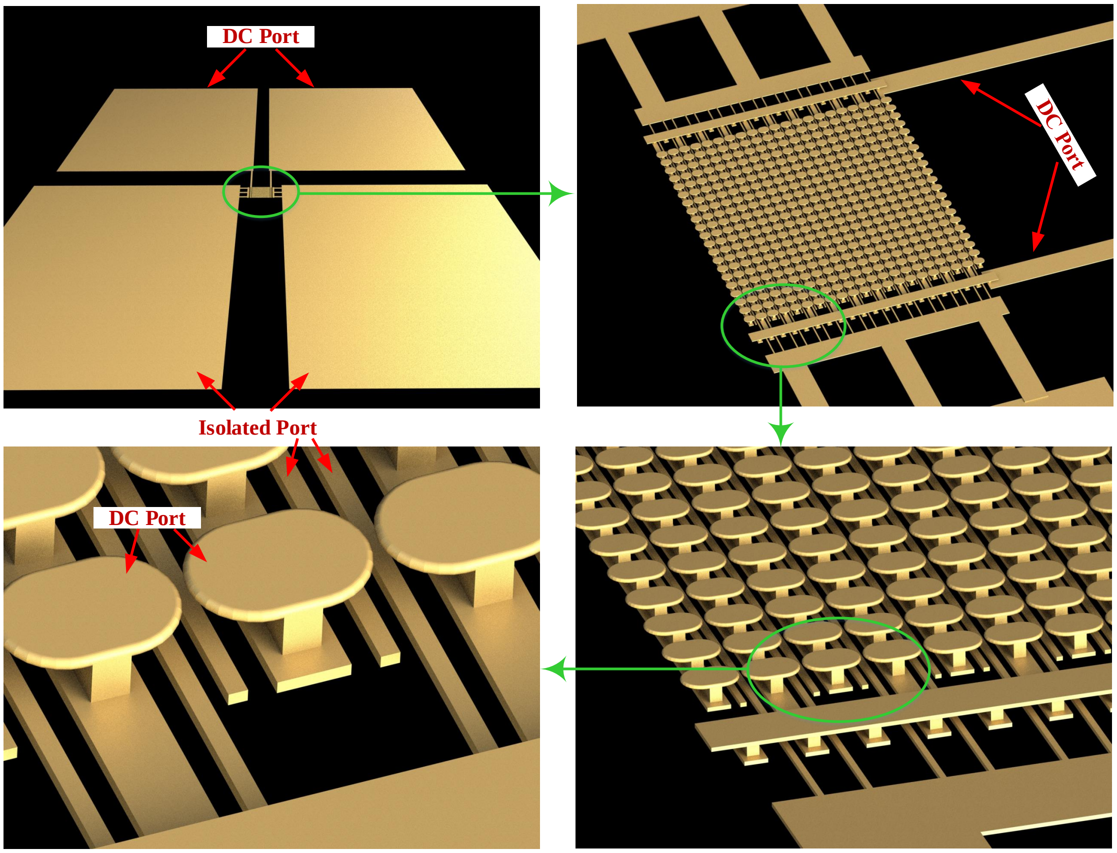


Figure S.3. The designed device with two electrical ports. Mushroom rows are to be biased with alternating polarities, using the two airbridges on the sides, to form the suspended port. The parallel strips on the substrate, below the gaps between the mushrooms, form the flat port.

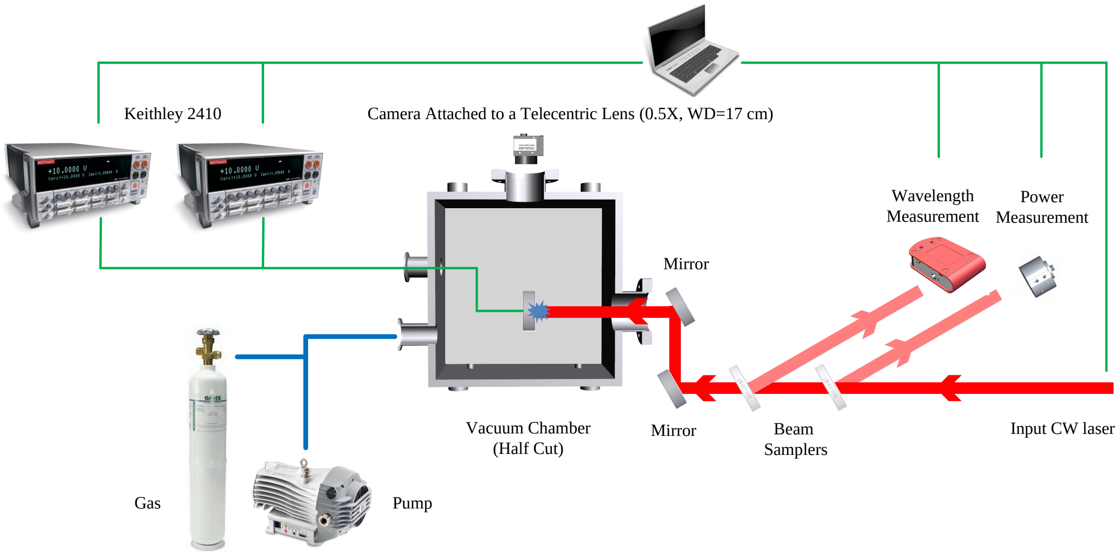


Figure S.4. The measurement setup.

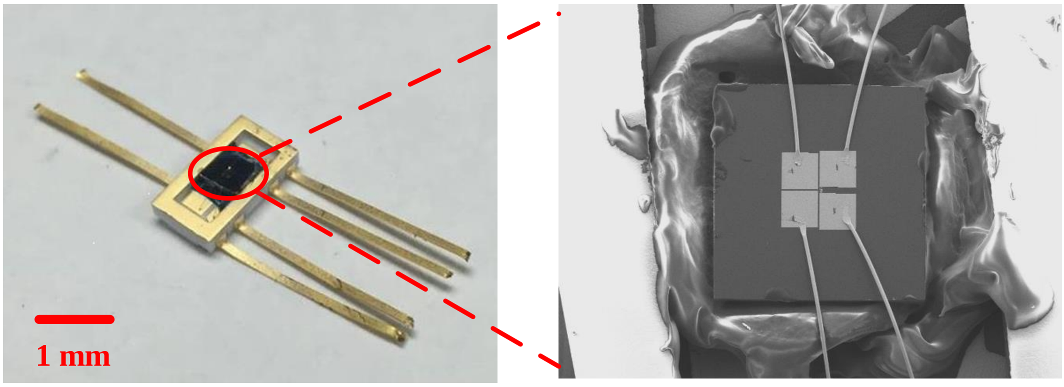


Figure S.5. A device installed and wire-bonded in the package (left) and the SEM picture of the wirebonded device (right).

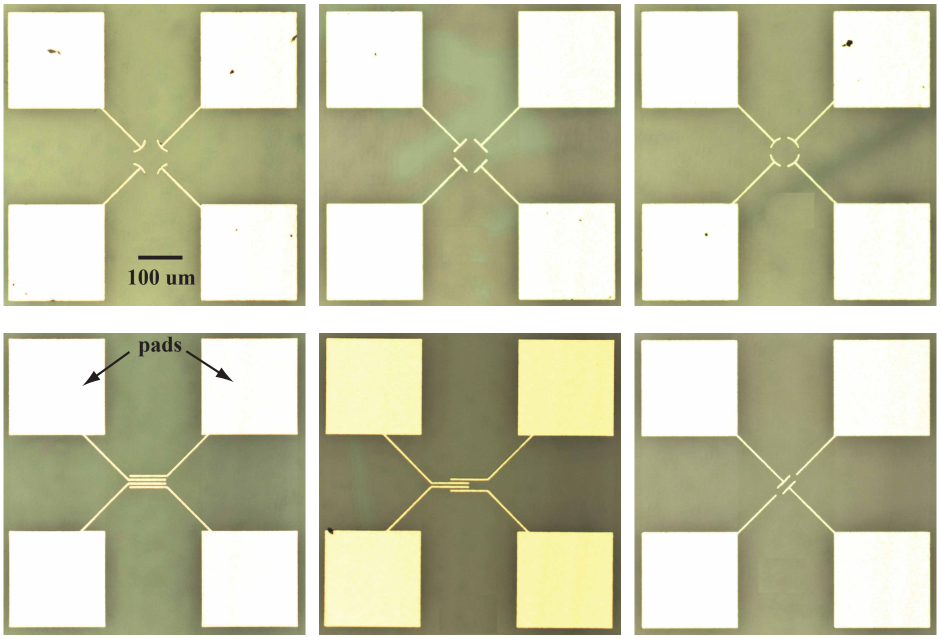


Figure S.6. Fabricated non-resonant flat structures on quartz substrate.

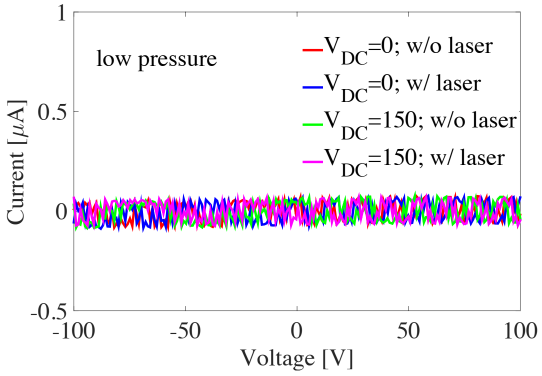


Figure S.7. I-V curves of the non-resonant flat structures.

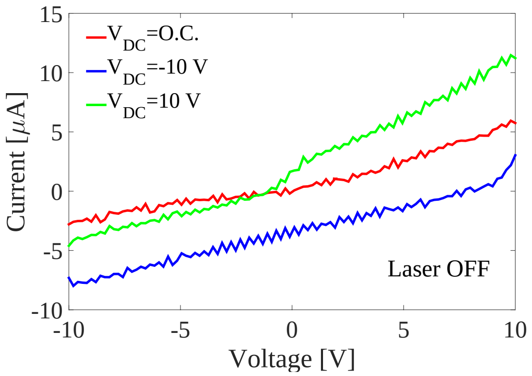


Figure S.8. I-V curves of the flat port without the laser illumination. The pressure was 0.1 $mTorr$.
